# Supplementary material for: Learning Equilibria in Adversarial Team Markov Games: A Nonconvex-Hidden-Concave Min-Max Optimization Problem
Source: arXiv:2410.05673 source file (2024-10-08)
Supplement: Supplementary file 1 [file marginalia.tex]

\subsection{Additional Auxiliary Claims}
\label{sec:marginalia}

For the sake of readability, this section contains some simple and standard claims we used earlier in our proofs, but are only stated here.

\begin{fact}
    \label{fact:boungrad}
    Let $f : \calX \ni \Vec{x} \mapsto \R$ be an $L$-Lipschitz continuous and differentiable function. Then,
    \begin{equation}
        \max_{\Vec{x} \in \calX} \|\nabla_{\Vec{x}} f(\Vec{x}) \| \leq L.
    \end{equation}
\end{fact}

\begin{fact}[Projection operator is nonexpansive]
    \label{fact:nonexpansive}
    Let $\calX \subseteq \R^d$ be a nonempty, convex and compact set. Further, let $\proj{\calX}: \R^d \rightarrow \calX $ be the Euclidean projection operator defined as $\proj{\calX}: \R^d \ni \vy \mapsto \frac{1}{2} \argmin_{\vx \in \calX}\| \vx - \vy \|^2 $. Then, for any $\vx, \vy \in \R^d$,
    \begin{equation}
        \| \proj{\calX}{\vx} - \proj{\calX}{\vy} \| \leq \| \vx - \vy\|.
    \end{equation}.
    \label{fact:proj-nonexpansive}
\end{fact}

In the rest of the claims, we are implicitly---for the sake of readability---fixing an adversarial team Markov game $(\calS, \calA, \calB, r, \pr , \gamma, \vrho)$.

\begin{claim}
    Consider any joint stationary policy $\policy{}\in \Pi$. For any $\gamma \in [0,1)$, the matrix $\mat{I} - \gamma \pr(\policy{})$ is invertible.
    \label{claim:iminusp-invertible}
\end{claim}

% \paragraph{Vector/matrix form of the discounted visitation distribution}
\begin{claim} Let $\policy{} \in \Pi$ be a joint stationary policy. The value vector $\vec{V} \in \R^{S}$ can be expressed as
    \begin{equation}
        \vec{V} = \big( \mat{I} - \gamma \mat{\pr}(\policy{}) \big)^{-1} \vr(\policy{}),
    \end{equation}
    where $\vr(\policy{})$ denotes the per-state reward under policy $\policy{}$.
    \label{fact:value-from-matrix}
\end{claim}
\begin{proof}
    For any state $s \in \calS$,
    \begin{equation}
        V_{s}(\policy{}) = \vr(\policy{}) + \gamma \pr(\policy{}) + \gamma^2 \pr^2(\policy{}) + \dots = \sum_{t=0}^\infty \gamma^t \pr^t(\policy{}) \vr(\policy{}). 
    \end{equation}
    But, given that the matrix $\mat{I} - \gamma \pr(\policy{})$ is invertible (\Cref{claim:iminusp-invertible}), we have
    \begin{equation}
        \sum_{t=0}^\infty \gamma^t \pr^t(\policy{}) = \big( \mat{I} - \gamma \pr (\policy{})\big)^{-1},
    \end{equation}
    and the claim follows.
\end{proof}

\begin{claim}
    \label{fact:visitation}
    Consider a stationary joint policy $\policy{} \in \Pi$. The discounted visitation measure $d_{\vrho}^{\policy{}}(s)$ can be expressed as
    \begin{equation}
        \left( {\vd^{\policy{}}_{\vrho}}\right)^\top = \vrho^\top \big(\mat{I} - \gamma \pr(\policy{}) \big)^{-1}.
    \end{equation}
\end{claim}

\begin{claim}
    \label{claim:visitation-and-value}
    Consider a stationary joint strategy $(\vx, \vy) \in \calX \times \calY$, and the visitation measure $\vd^{\px, \py}_{\vrho}$, under some initial distribution $\vrho \in \Delta(\calS)$. Then, the value function can be expressed as
    \begin{equation}
        V_{\vrho} = \sum_{s\in\calS} d_{\vrho}^{\px, \py}(s) r(s,\px,\py).
    \end{equation}
\end{claim}
\begin{proof}
    By definition of $\vd^{\px, \py}_{\vrho}$, we have that for any $s \in \calS$,
    \begin{equation}
        d_{\vrho}^{\px,\py}(s) = \sum_{\bar{s}\in\calS} \rho(\bar{s}) \sum_{t=0}^{\infty} \gamma^t \pr\left(s\step{t}=s ~\big|~ \px, \py, s\step{0} = \bar{s}\right).
    \end{equation}
    Similarly, the value function can be written as
    \begin{align}
        V_{\vrho}(\px, \py) = \sum_{s \in \calS} \sum_{\bar{s} \in \calS} \rho(\bar{s}) \sum_{t=0}^{\infty} \gamma^t \pr\left(s\step{t}=s ~\big|~ \px, \py, s\step{0} = \bar{s}\right) r(s, \px, \py) = \sum_{s\in\calS} d_{\vrho}^{\px, \py}(s) r(s, \px, \py).
    \end{align}
\end{proof}

\begin{claim}
    Let $\policy{} \in \Pi$ be a joint stationary policy, $\vr(\policy{})$ be the reward vector under $\policy{}$, and $\vv, \vc \in \R^S$. If $\vr (\policy{}) + \gamma \pr(\policy{}) \vv \leq \vv  + \vc$, then it holds that
    \begin{equation}
        \vec{V}( \policy{} ) \leq \vv + \big( \mat{I} - \gamma \pr(\policy{}) \big)^{-1}\vc.
    \end{equation}
    Similarly, if $\vr (\policy{}) + \gamma \pr(\policy{}) \vv \geq \vv  + \vc$, then it holds that 
    \begin{equation}
    \vec{V}( \policy{} ) \geq \vv + \big( \mat{I} - \gamma \pr(\policy{}) \big)^{-1}\vc.    
    \end{equation}
    \label{claim:vec-inequality}
\end{claim}

\begin{proof}
    Suppose that $\vr (\policy{}) + \gamma \pr(\policy{}) \vv \leq \vv  + \vc$. Applying recursively this inequality, it follows that
    \begin{equation}
        \sum_{t=0}^\infty \gamma^t \pr^{t}(\policy{}) \vr(\policy{}) -          \sum_{t=0}^\infty \gamma^t \pr^{t}(\policy{}) \vc \leq \vv.  
    \end{equation}
    Combining this bound with \Cref{claim:iminusp-invertible,fact:value-from-matrix} implies that
    \begin{equation}
        \vec{V}(\policy{}) - \Big( \mat{I} - \gamma \pr(\policy{}) \Big)^{-1} \vc \leq \vv.
    \end{equation}
    The case where $\vr (\policy{}) + \gamma \pr(\policy{}) \vv \geq \vv  + \vc$ admits an analogous proof.
\end{proof}

\begin{claim}
    \label{claim:stratequiv}
    Consider an adversarial team Markov game $\calG$. Altering all the rewards by adding an additive constant $c\in\R$ yields a \emph{strategically-equivalent} game $\calG'$: any $\epsilon$-approximate Nash equilibrium in $\calG'$ is also an $\epsilon$-approximate Nash equilibrium in $\calG$, and \emph{vice versa}.
\end{claim}
\begin{proof}
    By assumption, $r'(s,\va, b) = r(s,\va, b) + c $ for any $(s, \vec{a}, b) \in \calS \times \calA \times \calB$. Let $V'_{\vrho}$ be the value function in $\calG'$. Then, for all $(\px, \py) \in \calX \times \calY$,
    \begin{align}
        V'_{\vrho} (\px, \py )  &= \vrho^\top \left( \mat{I} - \gamma \pr(\px, \py) \right)^{-1} \vr'(\px, \py) \\
        &= \vrho^\top \left( \mat{I} - \gamma \pr(\px, \py) \right)^{-1} ( \vr(\px, \py) + c \cdot \vone ) \\
        &= V_{\vrho}(\px, \py)  + \frac{c}{1-\gamma}.
    \end{align}
    Thus, our claim follows immediately from the definition of Nash equilibria (\Cref{def:Nash}).
\end{proof}

\iffalse
Now let $(\hat{\px}, \hat{\py}) \in \calX \times \calY$ be an $\epsilon$-approximate NE of game $\calG$. Then, by definition,
    \begin{align}
        &V_{\vrho}(\hat{\px}, \hat{\py}) \geq V_{\vrho}(\hat{\px}, \py) - \epsilon, 
        ~\forall \py \in \calY\\
        &V_{\vrho}(\hat{\px}, \hat{\py}) \leq V_{\vrho}\left( ({\px}_k; \hat{\px}_{-k}), \hat{\py}\right) + \epsilon,
        ~\forall \px \in \calX_{k}.
    \end{align}
    Then, it is direct to see that the following inequalities hold as well:
    \begin{align}
        &V'_{\vrho}(\hat{\px}, \hat{\py}) \geq V'_{\vrho}(\hat{\px}, \py) - \epsilon, ~\forall \py \in \calY\\
        &V'_{\vrho}(\hat{\px}, \hat{\py}) \leq V'_{\vrho}\left( ({\px}_k; \hat{\px}_{-k}), \hat{\py} \right) + \epsilon,
        ~\forall \px \in \calX_{k}.
    \end{align}
    \textit{I.e.}, every $\epsilon$-approximate NE of $\calG$ is also an $\epsilon$-approximate NE of $\calG'$.
    
    Conversely, assuming $(\hat{\px}, \hat{\py})$ is an $\epsilon$-approximate NE of game $\calG'$ and subtracting $ \frac{1}{1-\gamma}c$ from both sides of the equilibrium inequalities implies that the aforementioned profile is also an $\epsilon$-approximate NE of the game $\calG$.
\fi

\begin{claim}
    \label{claim:rho-ul}
    Let $\policy{} \in \Pi$ be a joint stationary policy, and $\vd^{\policy{}}_{\vrho}$ be the induced visitation measure. Then, for every $s \in \calS$,
         $$ \rho(s) \leq d^{\policy{}}_{\vrho}(s) \leq \frac{1}{1 - \gamma}.$$
\end{claim}
\begin{proof}
This is an immediate consequence of the definition of $d^{\policy{}}_{\vrho}$; in particular,
\begin{equation}
    d^{\policy{}}_{\vrho}(s) =\sum_{\bar{s} \in \calS }\rho(\bar{s}) \sum_{t=0}^{\infty} \gamma^t { \pr} (s\step{t} = s | \policy{}, s\step{0} = \bar{s}) \leq \sum_{\bar{s} \in \calS} \rho(\bar{s}) \sum_{t=0}^\infty \gamma^t = \frac{1}{1 - \gamma},
\end{equation}
and 
\begin{equation}
    d^{\policy{}}_{\vrho}(s) =\sum_{\bar{s} \in \calS }\rho(\bar{s}) \sum_{t=0}^{\infty} \gamma^t { \pr} (s\step{t} = s | \policy{}, s\step{0} = \bar{s}) \geq \rho(s) \sum_{t=0}^{\infty} \gamma^t { \pr} (s\step{t} = s | \policy{}, s\step{0} = s) \geq \rho(s).
\end{equation}
\end{proof}

\begin{claim}
    \label{claim:V-bounds}
    Suppose that the reward function takes values in $[m_r, M_r]$, for some $m_r, M_r > 0$. Then, for any stationary joint policy $\policy{} \in \Pi$ and every state $s \in \calS$,
    \begin{equation}
        \frac{\minrew}{1-\gamma}\leq V_s(\policy{}) \leq \frac{\maxrew}{1-\gamma}.
    \end{equation}
\end{claim}

\begin{proof}
    By the definition of the value function in~\eqref{eq:value-func-def}, we have
    \begin{equation}
        V_s(\policy{}) \leq \maxrew + \gamma \maxrew + \gamma^2 \maxrew + \cdots = \frac{1}{1-\gamma} \maxrew,
    \end{equation}
    for any $s \in \calS$. Similarly, we conclude that
    \begin{equation}
       V_s(\policy{}) \geq \frac{1}{1-\gamma} \minrew.
    \end{equation}
\end{proof}

\begin{claim}
    \label{claim:various-bounds}
    Let an adversarial team Markov game $\calG$, two team policies $\tilde{\px}, \tilde{\px}$ and quantities $R_b(\cdot, \cdot), P_b(\cdot| s, \cdot), v(s)$ quantities defined in \pref{prog:xinlp}.
    The following inequalities hold:
    \begin{enumerate}
        \item $\left| r\left(s, \tilde{\px}, b \right) - r\left(s, \hat{\px}, b \right) \right| \leq \sqrt{\sum_{k=1}^n A_k} \| \tilde{\px} - \hat{\px} \|$, for any $(s,b) \in \calS \times \calB$; \label{item:reward}
    \item \label{item:prob} $ \left|  \sum_{s' \in \calS} \Big( \pr\left(s'|s,  \tilde{\px}, b \right) - \pr \left(s'|s, \hat{\px},b \right) \Big)
             \tilde{v}(s')  \right| \leq  \frac{S}{1-\gamma} \sqrt{\sum_{k=1}^n A_k} \|\tilde{\vx} - \hat{\vx}\|$, for any $(s,b) \in \calS \times \calB$;
    \item \label{item:val} $\left| \tilde{v}(s) - \hat{v}(s) \right| \leq L \| \tilde{\px} - \hat{\px}\|$, for any $s \in \calS$; and
    \item \label{item:last} $\left|  \sum_{s' \in \calS}  \pr \left(s'|s, \hat{\px}, b \right) \big( \tilde{v}(s') - \hat{v}(s') \big)  \right| \leq S  L \| \tilde{\px} - \hat{\px}\|$, for any $(s,b) \in \calS \times \calB$.
    \end{enumerate}
\end{claim}
\begin{proof} We briefly note how the bounds are derived:

    \begin{itemize}
        \item We first establish \Cref{item:reward}. Fix any pair $(s,b) \in \calS \times \calB$. By definition, we have
        \begin{equation}
            r(s, \tilde{\vx}, b) = \E_{\vec{a} \sim \tilde{\vx}}[r(s, \vec{a}, b)] = \sum_{(a_1, \dots, a_n) \in \calA} r(s, \vec{a}, b) \prod_{k = 1}^n \tilde{x}_{k, s, a_k}.
        \end{equation}
        As a result, 
        \begin{align}
            |r(s, \tilde{\vx}, b) - r(s,\hat{\vx}, b)| &= \left| \sum_{(a_1, \dots, a_n) \in \calA} r(s, \vec{a}, b) \prod_{k = 1}^n \tilde{x}_{k, s, a_k} - \sum_{(a_1, \dots, a_n) \in \calA} r(s, \vec{a}, b) \prod_{k = 1}^n \hat{x}_{k, s, a_k} \right| \\
            &= \left| \sum_{(a_1, \dots, a_n) \in \calA} r(s, \vec{a}, b) \left( \prod_{k=1}^n \tilde{x}_{k, s, a_k} - \prod_{k=1}^n \hat{x}_{k, s, a_k} \right) \right|\\
            &\leq \sum_{(a_1, \dots, a_n) \in \calA} \left| \prod_{k=1}^n \tilde{x}_{k, s, a_k} - \prod_{k=1}^n \hat{x}_{k, s, a_k} \right| \label{eq:triangle} \\
            &\leq \sum_{k=1}^n \| \tilde{\vx}_{k,s} - \hat{\vx}_{k, s} \|_1 = \| \tilde{\vx}_s - \hat{\vx}_s \|_1 \leq \left( \sqrt{\sum_{k=1}^n A_k} \right) \| \tilde{\vx}_s - \hat{\vx}_s\|_2, \label{eq:sum-product}
        \end{align}
        where \eqref{eq:triangle} follows from the triangle inequality and the fact that $|r(s, \vec{a}, b)| \leq 1$, and \eqref{eq:sum-product} follows from the fact that the total variation distance between two product distributions is bounded by the sum of the total variations of each marginal distribution~\citep{Hoeffding58:Distinguishability}, as well as the fact that $\|\vx \|_1 \leq \sqrt{d} \|\vx\|_2$ for a vector $\vx \in \R^d$.
        
        \item \Cref{item:prob} follows analogously to \Cref{item:reward}, using the fact that $\tilde{v}(s') \leq \frac{1}{1 - \gamma}$ (by \Cref{claim:V-bounds} and \Cref{prop:phi-and-nlp}).
        \item For \Cref{item:val}, we begin by noting that $\hat{\vv}$ and $\tilde{\vv}$ are the unique optimal vectors of \pref{prog:xinlp} for $\hat{\px}$ and $\tilde{\px}$ respectively (recall \Cref{prop:phi-and-nlp}). Further, by \Cref{prop:phi-and-nlp}, we know that $\vrho^\top \hat{\vv} =\max_{\py \in \calY} V_{\vrho}(\hat{\px}, \py) = \phi( \hat{\px})$ and 
        $\vrho^\top \tilde{\vv} =\max_{\py \in \calY} V_{\vrho}(\tilde{\px}, \py) = \phi( \tilde{\px})$,
        for any $\vrho\in\Delta(\calS)$ of full support. As a result, \Cref{item:val} is a consequence of the fact that $\phi(\cdot)$ is $L$-Lipschitz continuous, which in turn follows since $V_{\vrho}$ is $L$-Lipschitz continuous (see \Cref{lem:smoothness} and \Cref{lem:max-weakly-convex}).
        
        \item Finally, \Cref{item:last} follows from \Cref{item:val} and the fact that 
        \begin{align}
            \left| \sum_{s' \in \calS} \pr(s' | s, \hat{\vx}, b) \right| &= \left| \sum_{s' \in \calS} \sum_{(a_1, \dots, a_n) \in \calA} \pr(s' | s, \vec{a}, b) \prod_{k=1}^n \hat{\vx}_{k, s, a_k} \right| \\
            &\leq \sum_{s' \in \calS} \sum_{(a_1, \dots, a_n) \in \calA} \prod_{k=1}^n \hat{\vx}_{k, s, a_k} = S,
        \end{align}
        for any fixed $(s,b) \in \calS \times \calB$, where the last bound follows from the triangle inequality and the normalization constraint of the product distribution: $\sum_{(a_1, \dots, a_n) \in \calA} \prod_{k=1}^n \hat{\vx}_{k, s, a_k} = 1$.
    \end{itemize}
\end{proof}

% \fk{
% $$\frac{1}{\ell(1 - \gamma)}\left((BSD + 1)\frac{1}{1-\gamma}(L_r + \gamma S \matlip \frac{\maxrew}{1-\gamma} + \gamma S \matlip + \gamma S L + L ) + 2 \right)$$
% }

% \fk{
% $$
%     \frac{1}{1-\gamma}
%     \left[ 4\ell + 
%     (BSD + 1) \left(L_r + \gamma S \matlip \frac{\maxrew}{1-\gamma} + \gamma S \matlip + \gamma S L + L \right)
%     \right]
% $$
% }

% e, g, a, b , s, b
