# Supplementary material for: Learning Equilibria in Adversarial Team Markov Games: A Nonconvex-Hidden-Concave Min-Max Optimization Problem
Source: arXiv:2410.05673 source file (2024-10-08)
Supplement: Supplementary file 2 [file coupled-constraints.tex]

\section{Coupled Constraint Minimax Optimization}

\subsection{Continuity Theorems}
\begin{theorem}[Continuity of the maximizers functions]
    
\end{theorem}
$$\vx \in \calX \subset \R^n, \vy \in \calY(\vx) \subseteq \calY\subset \R^m$$

\newcommand{\diam}{\mathrm{D}}

Consider $\vx_1, \vx_2$.
\begin{align}
    &\nabla f\paren{\vx_1, \vy_1^\star(\vx_1)}^\top\paren{\vy_1 - \vy_1^\star(\vx_1)}\leq 0, ~\quad \forall \vy_1 \in \calY(\vx_1)\\
    &\nabla f\paren{\vx_2, \vy_2^\star(\vx_2)}^\top\paren{\vy_2 - \vy_2^\star(\vx_2)}\leq 0, ~\quad \forall \vy_2 \in \calY(\vx_2)\
\end{align}

We now consider $\bar\vx$ that belong to the set $\bar\calY = \calY(\vx_1) \cup \calY(\vx_2)$. We manage to show that the two latter inequalities hold approximately for the union of the feasibility sets. 

For every $\vy_{1}\in\calY(\vx_1)$, we pick a $\bar{\vy}$ $\vx_2$ instead. \textit{I.e.}, $\|\bar\vy - \vy_1\| \leq L_{\calY} \|\vx_1 - \vx_2\|$. We can do this for all $\vy_1$, hence the approximate inequality will also hold for any $\bar\vy\in \bar{\calY}$. We choose $\bar\vy$ in the second inequality accordingly.

\begin{align}
    &\nabla f\paren{\vx_1, \vy^\star(\vx_1)}^\top\left(\bar\vy - \vy_1^\star(\vx_1)\right) \leq L_{\calY}\diam_{\calY} \|\vx_1 - \vx_2 \|, ~\quad \forall \bar\vy \in \bar\calY\\
    &\nabla f\paren{\vx_2, \vy_2^{\star}(\vx_2)}^\top\left(\bar\vy- \vy_2^\star(\vx_2)\right) \leq  L_{\calY}\diam_{\calY} \|\vx_1 - \vx_2 \|, ~\quad \forall \bar\vy \in \bar\calY\\
\end{align}

We plug in $\bar\vy \gets \vy_2^\star(\vx_2)$ and $\bar\vy \gets \vy_1^\star(\vx_1)$ accordingly,

\begin{align}
       &\nabla f\paren{\vx_1, \vy^\star(\vx_1)}^\top\left(\vy_2^\star(\vx_1) - \vy_1^\star(\vx_1)\right) \leq L_{\calY}\diam_{\calY} \|\vx_1 - \vx_2 \|, \\
    &\nabla f\paren{\vx_2, \vy_2^{\star}(\vx_2)}^\top\left(\vy_1^\star(\vx_1)- \vy_2^\star(\vx_2)\right) \leq  L_{\calY}\diam_{\calY} \|\vx_1 - \vx_2 \|.\\ 
\end{align}

Adding the two inequalities results in,
\begin{align}
    \Big(\nabla f \paren{ \vx_1, \vy_1^{\star}(\vx_1) } - \nabla f\paren{\vx_2, \vy_2^\star(\vx_2)}\Big)^\top\left(\vy_2^\star(\vx_1) - \vy_1^\star(\vx_1)\right) \leq2 L_{\calY}\diam_{\calY} \|\vx_1 - \vx_2 \| 
    \label{approx-ineq-1}
    % 
    % 
    % \left(\vy_2^\star(\vx_1)- \vy_2^\star(\vx_2)\right) \leq  L_{\calY}\diam_{\calY}
\end{align}

Since $f(\vx, \cdot)$ is $\nu$-strongly concave for all $\vx$,
\begin{align}
    \left( \vy_1 - \vy_1^\star(\vx_1) \right)^\top     
    \Big(\nabla f\paren{\vx_1, \vy_1 } - \nabla f \paren{ \vx_1, \vy_1^{\star}(\vx_1) } \Big) + \nu \| \vy_1 - \vy_1^\star(\vx_1)\|^2 \leq 0, ~\forall \vy_1 \in \calY(\vx_1).
\end{align}

We again want to inflate the feasibility set into $\bar\vy \in \bar \calY$. We remind the reader that for every $\bar\vy$, it holds that there exists $\vy_1$ s.t. $\| \bar\vy - \vy_1\| \leq L_{\calY} \|\vx_1 - \vx_2 \| $. 

\begin{align}
    &\left( \vy_1+ (\bar\vy - \bar\vy)- \vy_1^\star(\vx_1) \right)^\top     
    \Big(\left( \nabla f(\vx_1, \vy_1) +\left( \nabla f(\vx_1, \bar\vy) - \nabla f(\vx_1, \bar\vy) \right) \right) - \nabla f \paren{ \vx_1, \vy_1^{\star}(\vx_1) } \Big)\\ &+ \nu \| \vy_1 + (\bar\vy - \bar\vy) - \vy_1^\star(\vx_1)\|^2 \leq 0, \quad \forall \vy_1 \in \calY(\vx_1).
\end{align}

We develop the latter display,
\begin{align}
    0 \geq &\underbrace{\left( \bar\vy - \vy_1^\star(\vx_1) \right)^\top     
    \Big(\left( \nabla f(\vx_1, \vy_1) +\left( \nabla f(\vx_1, \bar\vy) - \nabla f(\vx_1, \bar\vy) \right) \right) - \nabla f \paren{ \vx_1, \vy_1^{\star}(\vx_1) } \Big)}_{\Omega_1} \\
    &+\underbrace{ \nu \| \vy_1 + (\bar\vy - \bar\vy) - \vy_1^\star(\vx_1)\|^2}_{\Omega_2}\\
    &+\underbrace{(\vy_1  - \bar\vy)^\top     
    \Big(\left( \nabla f(\vx_1, \vy_1) +\left( \nabla f(\vx_1, \bar\vy) - \nabla f(\vx_1, \bar\vy) \right) \right) - \nabla f \paren{ \vx_1, \vy_1^{\star}(\vx_1) } \Big)}_{\Omega_3} 
\end{align}

We will bound $\Omega_1, \Omega_2,$ and $\Omega_3$ separately.
\begin{itemize}
    \item 
For $\Omega_1$:
\begin{align}
\left( \bar\vy - \vy_1^\star(\vx_1) \right)^\top     
        \Big( \nabla f(\vx_1, \vy_1)  - \nabla f(\vx_1, \bar\vy) \Big) &\leq \diam_{\calY}  \ell \|\vy_1 - \bar{\vy} \| \\  &\leq \diam_{\calY}  \ell L_{\calY} \norm{\vx_1 - \vx_2}
\end{align}

\item For $\Omega_2$, we get the following equality:
\begin{align}
     \| \vy_1 + (\bar\vy - \bar\vy) - \vy_1^\star(\vx_1)\|^2 = \| \vy_1 - \bar\vy\|^2 + \| \bar\vy - \vy^\star_1(\vx_1) \|^2 + 2\inprod{\vy_1 - \bar\vy}{\bar\vy - \vy^\star_1(\vx_1)}
\end{align}
Since all but the last term are non-negative, we need to bound the last term only,
\begin{align}
    \left|\inprod{\vy_1 - \bar\vy}{\bar\vy - \vy^\star_1(\vx_1)}\right| \leq  L_{\calY}\|\vx_1 - \vx_2\| \diam_{\calY}
\end{align}
Resulting in the bound, 
\begin{align}
    - 2 \nu L_{\calY}\|\vx_1 - \vx_2\| \diam_{\calY}  +  \nu \|\bar\vy - \vy^\star(\vx_1) \|^2 \leq \Omega_2.
\end{align}

\item For $\Omega_3$:
\begin{align}
    \Omega_3 = (\vy_1  - \bar\vy)^\top     
    \Big(  - \nabla f(\vx_1, \vy_1)  + \nabla f(\vx_1, \vy_1^\star(\vx_1)) \Big)
\end{align}
Hence,
\begin{align}
    |\Omega_3| \leq  L_{\calY}\|\vx_1 - \vx_2\| \ell \diam_{\calY}
\end{align}

Finally, putting the bounds of $\Omega_1, \Omega_2, \Omega_3$, 
\begin{align}
    \left( \bar{\vy} - \vy_1^\star(\vx_1)\right)^\top \left( \nabla f(\vx_1, \bar\vy) - \nabla f(\vx_1, \vy^\star(\vx_1) \right) + \nu \| \bar\vy - \vy_{1}^\star(\vx_1)\|^2 \leq L' \|\vx_1 - \vx_2\|,
    \label{penultimate-ineq-for-reg-max}
\end{align}
where $L' \defeq \paren{ 2 L_{\calY}\ell \diam_{\calY} + 2 \nu L_{\calY} }$

Concluding, we will plug $\bar\vy \gets \vy_2^\star(\vx_2)$ in \eqref{penultimate-ineq-for-reg-max} to get,
\begin{align}
    \left( {\vy}_2^\star(\vx_2) - \vy_1^\star(\vx_1)\right)^\top \left( \big(\vr(\vx_1) - \nu  {\vy}_2^\star(\vx_2) \big) - \big(\vr(\vx_1) - \nu\vy^\star(\vx_1) \big) \right) + \nu \|  {\vy}_2^\star(\vx_2) - \vy_{1}^\star(\vx_1)\|^2~~&\\  \leq L' \|\vx_1 - \vx_2\|& \label{approx-ineq-2}
\end{align}
\end{itemize}

Combining \eqref{approx-ineq-1} and \eqref{approx-ineq-2},

\begin{align}
     \nu \|  {\vy}_2^\star(\vx_2) - \vy_{1}^\star(\vx_1)\|^2 &\leq \left( {\vy}_2^\star(\vx_2) - \vy_1^\star(\vx_1)\right)^\top
     \Big(\nabla f\paren{\vx_2, \vy_2^\star(\vx_2)}- \nabla f\paren{\vx_1, \vy_2^\star(\vx_2)} \Big)
     + L''\| \vx_1 - \vx_2\|\\
     &\leq   \|\vy_2^{\star}(\vx_2) - \vy_1^{\star}(\vx_1)\| \ell \|\vx_1 - \vx_2\| + L''\|\vx_1 - \vx_2\|
\end{align}

$L'' = 2L_{\calY}\diam_{\calY} + L'$.

For convenience we can set $\lambda = \norm{{\vy}_2^\star(\vx_2) - \vy_{1}^\star(\vx_1)}$ and $\chi = \norm{\vx_1 - \vx_2}$:
\begin{align}
    &\nu \lambda^2 \leq \ell \lambda \chi +  L'' \chi 
\end{align}
% Let, $\xi \defeq \frac{\nu}{\max\{c_1,c_2\} \max\{\chi\}}$,
In general, for the quadratic inequality $\alpha \lambda^2 \leq \beta\lambda \chi + \gamma \chi$, with $\alpha, \beta, \gamma, \chi > 0$ it should be the case that,
\begin{align}
    0\leq \lambda\leq \frac{\chi + \sqrt{\chi + (4\alpha\gamma + \beta^2\chi) } }{2\alpha}
\end{align}

First, we attempt to prove that the maximizers are Lipschitz continuous. \textit{I.e.}, we attempt to find a $c>0$ such that the following inequality will hold, 
\begin{align}
   \frac{\chi + \sqrt{\chi(4\alpha\gamma + \beta^2\chi) } }{2\alpha}
 \leq  c\chi
\end{align}

$4\alpha\gamma \geq \beta^2\chi$

\begin{align}
    \frac{\chi + \sqrt{\chi(\beta^2\chi + \beta^2\chi)} }{2\alpha} \leq c \chi
\end{align}

But $4\alpha < \beta^2\chi$
\begin{align}
    \frac{\chi + \sqrt{8\chi\alpha\gamma} }{2\alpha} \leq c \chi
\end{align}

\begin{align}
    \|\vy_1^\star(\vx_1) - \vy_2^\star(\vx_2)\| \leq \bar L \sqrt{ \| \vx_1 - \vx_2 \|}
\end{align}

Solve the following inequality for $c$:
\begin{align}
        \frac{\chi + \sqrt{\chi(4\alpha\gamma + \beta^2\chi) } }{2\alpha} \leq c \sqrt{\chi}
\end{align}

For $\chi > 0$
\begin{align}
    c \geq \frac{\chi + \sqrt{\chi(4\alpha\gamma + \beta^2\chi) } }{2\alpha \sqrt{\chi}}  = \frac{\sqrt{\chi}}{2\alpha} + \frac{\sqrt{4\alpha\gamma + \beta^2\chi}}{2\alpha}
\end{align}

\begin{align}
    \max_{X \geq \chi\geq 0} \left\{ \frac{\sqrt{\chi}}{2\alpha} + \frac{\sqrt{4\alpha\gamma + \beta^2\chi}}{2\alpha} \right\} = \frac{\sqrt{X}}{2\alpha} + \frac{\sqrt{4\alpha\gamma  +\beta^2 X}}{2\alpha}
\end{align}

For $\chi = 0$, the inequality holds trivially. $c \gets \frac{1}{\alpha} \sqrt{2\beta^2 X + 4\alpha \gamma } $
