# Supplementary material for: Learning Equilibria in Adversarial Team Markov Games: A Nonconvex-Hidden-Concave Min-Max Optimization Problem
Source: arXiv:2410.05673 source file (2024-10-08)
Supplement: Supplementary file 3 [file continuity-lemmas.tex]

\subsection{Maximizer Continuity}
\input{sections/appendix/reg-max-continuity}
